# Supplementary material for: Online learning over a finite action set with limited switching
Source: arXiv:1803.01548 source file (2018-06-13)
Supplement: Supplementary file 2 [file appendix_hp_sc_lb.tex]

% !TEX root = colt2018-switching.tex

\section{Proof of Theorem~\ref{thm:hp-sc-lb}: lower bound on high-probability bounds for PFE}\label{app:hp-sc-lb}
\textbf{\textcolor{red}{\textbf{TODO: KUNAL}}}
